# Supplementary material for: Multi-modal Test-time Adaptation via Adaptive Probabilistic Gaussian Calibration
Source: arXiv:2604.19093 source file (2026-04-21)
Supplement: Supplementary file 1 [file x_appendix.tex]

\clearpage
\setcounter{page}{1}
\maketitlesupplementary

\section*{A. Proofs of Theorems}
\subsection*{A.1 Derivation of Gaussian Discriminant Functions}
We consider GDA under the assumption that the category-conditional
distributions are multivariate Gaussians with a shared covariance matrix $\boldsymbol{\Sigma}$:

\begin{align}
    p(\boldsymbol{z}\mid c)
& = \mathcal{N}(\boldsymbol{z}; \boldsymbol{\mu}_c, \boldsymbol{\Sigma})\\
& = \frac{1}{\sqrt{(2\pi)^d |\boldsymbol{\Sigma}|}}
\exp\!\left( -\frac{1}{2}(\boldsymbol{z}-\boldsymbol{\mu}_c)^\top
\boldsymbol{\Sigma}^{-1}(\boldsymbol{z}-\boldsymbol{\mu}_c) \right),
\end{align}
where $\boldsymbol{\mu}_c$ denotes the category mean.

By Bayes’ theorem, the posterior of category $c$ given $\boldsymbol{z}$ is
\begin{equation}
p(c\mid \boldsymbol{z})
= \frac{p(\boldsymbol{z}\mid c)p(c)}{\sum_{c'=1}^{C}p(\boldsymbol{z}\mid c')p(c')}
= \frac{p(\boldsymbol{z}\mid c)\,\pi_c}{\sum_{c'=1}^{C}p(\boldsymbol{z}\mid c')\,\pi_{c'}},
\end{equation}
where $\pi_c = p(c)$ denotes the prior of category $c$.
For prediction we only need
\(
\arg\max_c p(c\mid\boldsymbol{z}),
\)
which is equivalent to
\begin{equation}
\arg\max_c p(\boldsymbol{z}\mid c)\,\pi_c.
\end{equation}
Taking logarithms does not change the maximizer and turns the product into a
sum, which is both numerically more stable and algebraically simpler. We
therefore define the (unnormalized) log-posterior
\begin{equation}
\ell_c(\boldsymbol{z})
:= \log p(\boldsymbol{z}\mid c) + \log \pi_c.
\end{equation}

Substituting the Gaussian density yields
\begin{align}
\ell_c(\boldsymbol{z})
&= \log \frac{1}{\sqrt{(2\pi)^d |\boldsymbol{\Sigma}|}}
   -\frac{1}{2}(\boldsymbol{z}-\boldsymbol{\mu}_c)^\top
      \boldsymbol{\Sigma}^{-1}(\boldsymbol{z}-\boldsymbol{\mu}_c)
   + \log \pi_c \\
&= -\frac{d}{2}\log 2\pi
   -\frac{1}{2}\log|\boldsymbol{\Sigma}|  -\frac{1}{2}\boldsymbol{z}^\top\boldsymbol{\Sigma}^{-1}\boldsymbol{z}
   + \boldsymbol{\mu}_c^\top\boldsymbol{\Sigma}^{-1}\boldsymbol{z}
   - \frac{1}{2}\boldsymbol{\mu}_c^\top\boldsymbol{\Sigma}^{-1}\boldsymbol{\mu}_c
   + \log \pi_c.
\end{align}
Terms that do not depend on $c$ do not affect the softmax over categories and can be dropped.
Collecting the $c$-dependent terms gives

\begin{equation}
\ell_c(\boldsymbol{z})
\;\dot{=}\;
\boldsymbol{\mu}_c^\top\boldsymbol{\Sigma}^{-1}\boldsymbol{z}
- \frac{1}{2}\boldsymbol{\mu}_c^\top\boldsymbol{\Sigma}^{-1}\boldsymbol{\mu}_c
+ \log \pi_c
= \mathbf{w}_c^\top \boldsymbol{z} + b_c,
\end{equation}
where $\dot{=}$ denotes equality up to an additive term independent of $c$, and
\[
\mathbf{w}_c = \boldsymbol{\Sigma}^{-1}\boldsymbol{\mu}_c,\qquad
b_c = -\frac{1}{2}\boldsymbol{\mu}_c^\top\boldsymbol{\Sigma}^{-1}\boldsymbol{\mu}_c
      + \log \pi_c.
\]
Thus, under a shared covariance matrix, the GDA discriminant is linear in
$\boldsymbol{z}$, and the posterior is obtained via
\[
p(c\mid\boldsymbol{z})
= \text{Softmax}_c\bigl(\mathbf{w}_c^\top \boldsymbol{z} + b_c\bigr).
\]

% ----in our work----
In our work, we relax the shared-covariance assumption and allow each category
to have its own covariance matrix $\boldsymbol{\Sigma}_c$:
\begin{align}
    p(\boldsymbol{z}\mid c)
    &= \mathcal{N}(\boldsymbol{z}; \boldsymbol{\mu}_c, \boldsymbol{\Sigma}_c) \\
    &= \frac{1}{\sqrt{(2\pi)^d |\boldsymbol{\Sigma}_c|}}
    \exp\!\left( -\frac{1}{2}(\boldsymbol{z}-\boldsymbol{\mu}_c)^\top
    \boldsymbol{\Sigma}_c^{-1}(\boldsymbol{z}-\boldsymbol{\mu}_c) \right).
\end{align}

By the same derivation, the (unnormalized) log-posterior becomes
\begin{align}
g_c(\boldsymbol{z})
&= \log p(c) + \log p(\boldsymbol{z}\mid c) \\
&= -\frac{1}{2}\boldsymbol{z}^\top \boldsymbol{\Sigma}_c^{-1} \boldsymbol{z}
   + \boldsymbol{\mu}_c^\top \boldsymbol{\Sigma}_c^{-1}\boldsymbol{z} - \frac{1}{2}\boldsymbol{\mu}_c^\top \boldsymbol{\Sigma}_c^{-1}\boldsymbol{\mu}_c
   - \frac{1}{2}\log |\boldsymbol{\Sigma}_c|
   + \log \pi_c
   \;+\; \text{const},
\end{align}
which can be summarized as a quadratic discriminant
\begin{equation}
g_c(\boldsymbol{z})
\;\dot{=}\;
-\frac{1}{2}\boldsymbol{z}^\top \mathbf{A}_c \boldsymbol{z}
+ \mathbf{b}_c^\top \boldsymbol{z}
+ d_c,
\end{equation}
where
\begin{align}
\mathbf{A}_c &= \boldsymbol{\Sigma}_c^{-1},\\
\mathbf{b}_c &= \boldsymbol{\Sigma}_c^{-1}\boldsymbol{\mu}_c,\\
d_c &= - \frac{1}{2}\boldsymbol{\mu}_c^\top \boldsymbol{\Sigma}_c^{-1}\boldsymbol{\mu}_c
      - \frac{1}{2}\log |\boldsymbol{\Sigma}_c|
      + \log \pi_c.
\end{align}

Here the quadratic term $-\tfrac{1}{2}\boldsymbol{z}^\top \boldsymbol{\Sigma}_c^{-1}\boldsymbol{z}$
depends on the category index $c$, so $g_c(\boldsymbol{z})$ cannot be reduced
to a linear function of $\boldsymbol{z}$. The posterior is again obtained
by normalizing these scores with a softmax:
\begin{align}
    p(c\mid\boldsymbol{z})
= \text{Softmax}_c\bigl(g_c(\boldsymbol{z})\bigr).
\end{align}

\subsection*{A.2 Maximum-likelihood Estimation of Gaussian Parameters}
Since we model the category prior and category-conditional density as
\[
p(y=c)=\pi_c,\qquad \sum_{c=1}^C \pi_c = 1,
\]
\[
p(\boldsymbol{z}\mid y=c)
= \mathcal{N}(\boldsymbol{z};\boldsymbol{\mu}_c,\boldsymbol{\Sigma}_c),
\]
where each category $c$ is associated with its own mean $\boldsymbol{\mu}_c$ and covariance matrix $\boldsymbol{\Sigma}_c$, we estimate these parameters from a finite set of labeled feature vectors 
$\{(\boldsymbol{z}_i, y_i)\}_{i=1}^N$ with 
$\boldsymbol{z}_i \in \mathbb{R}^d$ and $y_i \in \{1,\dots,C\}$.
Let $\mathcal{I}_c = \{i: y_i=c\}$ and $N_c = |\mathcal{I}_c|$ denote
the index set and sample size of category $c$, respectively.
Under the i.i.d.\ assumption, the joint likelihood of all samples is
\begin{align}
\label{eq:gda-likelihood}
p(\{\boldsymbol{z}_i,y_i\}_{i=1}^N \mid \theta)
&= \prod_{i=1}^N p(y_i)\,p(\boldsymbol{z}_i\mid y_i)\\
&= \prod_{c=1}^C 
\Bigg[
\pi_c^{N_c}
\prod_{i\in\mathcal{I}_c}
\mathcal{N}(\boldsymbol{z}_i;\boldsymbol{\mu}_c,\boldsymbol{\Sigma}_c)
\Bigg],
\end{align}
where $\theta = \{\pi_c,\boldsymbol{\mu}_c,\boldsymbol{\Sigma}_c\}_{c=1}^C$ collects all
parameters.
Taking logarithms yields the log-likelihood
\begin{align}
\label{eq:gda-loglik}
\ell(\theta)
= \sum_{c=1}^C
\Bigg[
&N_c \log \pi_c
-\frac{N_c}{2}\log|\boldsymbol{\Sigma}_c|-\frac{1}{2}\sum_{i\in\mathcal{I}_c}
(\boldsymbol{z}_i-\boldsymbol{\mu}_c)^\top
\boldsymbol{\Sigma}_c^{-1}
(\boldsymbol{z}_i-\boldsymbol{\mu}_c)
\Bigg]
+ \text{const},
\end{align}
where the constant term does not depend on $\theta$ and can thus be omitted in the optimization.

% ----------------

Maximizing the log-likelihood with respect to $\theta$ yields closed-form solutions for all parameters.
For the category priors, we introduce a Lagrange multiplier to enforce 
$\sum_c \pi_c = 1$ and take the derivative of $\ell(\theta)$ with respect 
to $\pi_c$. The resulting stationarity condition equates the gradient to zero 
and yields
\begin{equation}
    \hat{\pi}_c = \frac{N_c}{N},
\end{equation}
meaning that the optimal prior of each category coincides with its empirical frequency.

For the category means, differentiating $\ell(\theta)$ with respect to 
$\boldsymbol{\mu}_c$ shows that the gradient is proportional to 
$\sum_{i\in\mathcal{I}_c} (\boldsymbol{z}_i - \boldsymbol{\mu}_c)$. 
Setting this gradient to zero imposes 
$\sum_{i\in\mathcal{I}_c} \boldsymbol{z}_i = N_c \boldsymbol{\mu}_c$, 
which directly leads to
\begin{equation}
    \hat{\boldsymbol{\mu}}_c
= \frac{1}{N_c}\sum_{i\in\mathcal{I}_c} \boldsymbol{z}_i.
\end{equation}

Finally, for the covariance matrices, we collect all terms in \eqref{eq:gda-loglik} that depend on $\boldsymbol{\Sigma}_c$ and differentiate the log-likelihood with respect to $\boldsymbol{\Sigma}_c^{-1}$.
The covariance-dependent part of the objective is determined jointly by the log-determinant term $N_c \log|\boldsymbol{\Sigma}_c|$ and the empirical scatter
$\sum_{i \in \mathcal{I}_c}
(\boldsymbol{z}_i - \boldsymbol{\mu}_c)
(\boldsymbol{z}_i - \boldsymbol{\mu}_c)^\top,$
and the first-order optimality condition yields the familiar closed-form estimator
\begin{align}
\hat{\boldsymbol{\Sigma}}_c
&= \frac{1}{N_c}
\sum_{i\in\mathcal{I}_c}
(\boldsymbol{z}_i-\hat{\boldsymbol{\mu}}_c)
(\boldsymbol{z}_i-\hat{\boldsymbol{\mu}}_c)^\top\\
&= \frac{1}{N_c}
\left(
\sum_{i\in\mathcal{I}_c}\boldsymbol{z}_i\boldsymbol{z}_i^\top
- N_c\,\hat{\boldsymbol{\mu}}_c\hat{\boldsymbol{\mu}}_c^\top
\right).
\end{align}
% --------------
To better accommodate the TTA setting, we do not store individual feature vectors but instead maintain, for each category $c$, the following sufficient statistics:
\[
N_c = |\mathcal{I}_c|,\qquad
\mathbf{S}_c = \sum_{i\in\mathcal{I}_c} \boldsymbol{z}_i,\qquad
\mathbf{Q}_c = \sum_{i\in\mathcal{I}_c} \boldsymbol{z}_i\boldsymbol{z}_i^\top,
\]
which compactly summarize the number of samples, the aggregated first-order moment, 
and the aggregated second-order moment of the features in category $c$.
These statistics can be updated over time by simply accumulating contributions from new samples.

% ----
Using these sufficient statistics, the maximum-likelihood estimates take the compact form
\begin{equation}
\label{eq:gda-mle-N-S-Q}
\hat{\pi}_c = \frac{N_c}{\sum_j N_j},\qquad
\hat{\boldsymbol{\mu}}_c = \frac{\mathbf{S}_c}{N_c},\qquad
\hat{\boldsymbol{\Sigma}}_c
= \frac{\mathbf{Q}_c}{N_c}
  - \hat{\boldsymbol{\mu}}_c \hat{\boldsymbol{\mu}}_c^\top.
\end{equation}

Thus, once the sufficient statistics $(N_c,\mathbf{S}_c,\mathbf{Q}_c)$ have been updated from the incoming stream, the Gaussian parameters $(\hat{\pi}_c,\hat{\boldsymbol{\mu}}_c,\hat{\boldsymbol{\Sigma}}_c)$ can be recovered without revisiting past samples.
This property is particularly beneficial in our streaming TTA scenario.

\begin{figure*}[t]
  \centering
  \includegraphics[width=\linewidth]{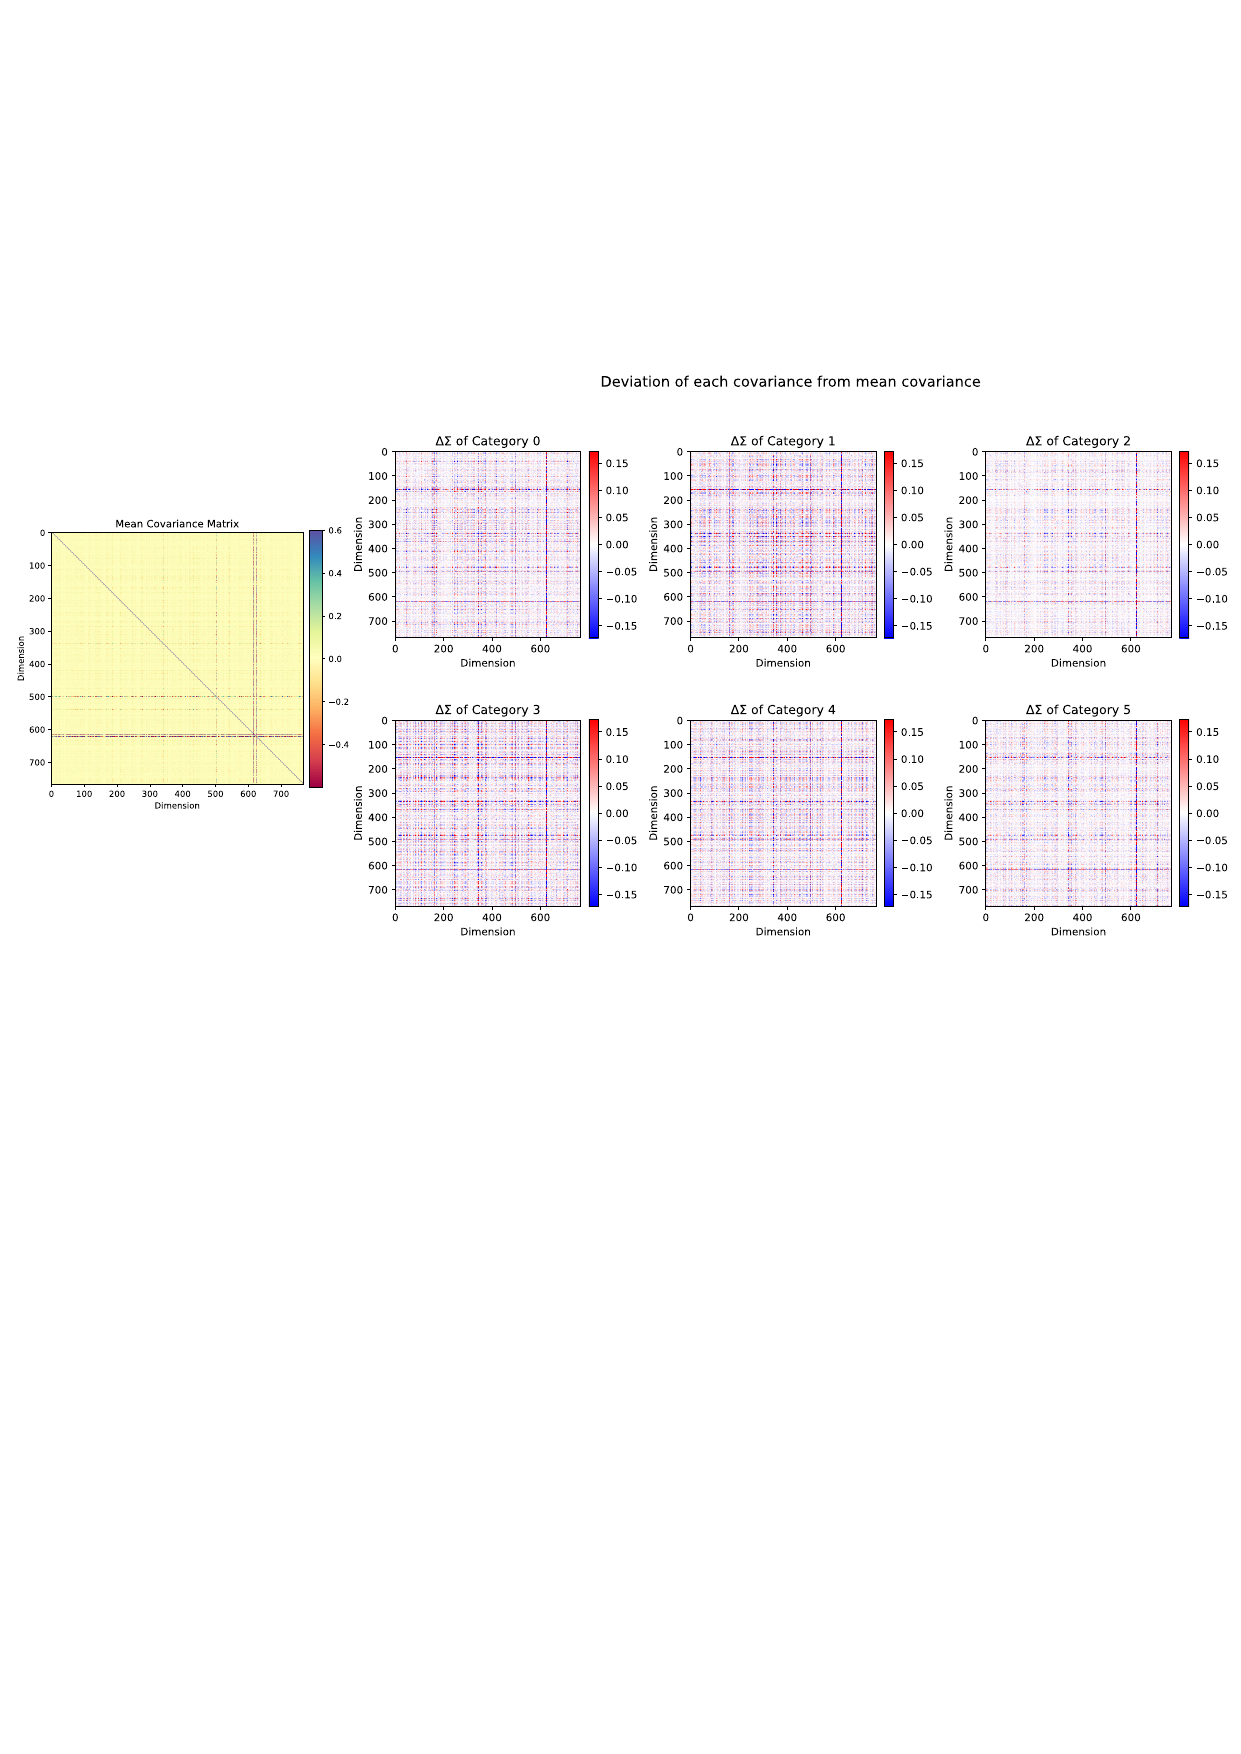}
\caption{Visualization of the average covariance and category-specific deviations of the Gaussian distributions.
The left panel shows the covariance matrix averaged over all categories. 
The right panels show the deviation matrices $\Delta \boldsymbol{\Sigma}_c = \boldsymbol{\Sigma}_c - \bar{\boldsymbol{\Sigma}}$ for the first six categories, where red (blue) entries indicate covariance values larger (smaller) than the global average.
}
  \label{fig:cov}
\end{figure*}

\section*{B. More Details about the Backbone}

Our audio-visual backbone is based on the CAV-MAE architecture \cite{gong2023contrastive} and consists of an audio encoder $\phi_1$, a video encoder $\phi_2$, and a joint encoder $\mathcal{F}$. The audio encoder $\phi_1$ splits the Mel-spectrogram into patches and maps them into an audio token sequence, while the video encoder $\phi_2$ divides video frames into image patches and maps them into a visual token sequence. 
These token sequences are then fed into the joint encoder $\mathcal{F}$, which models three perspectives: audio-only, video-only, and multi-modal. 
The joint encoder shares the multi-head self-attention and feed-forward parameters across these perspectives, while maintaining separate LayerNorm modules for each view. 
In this way, different modalities and their fusion are embedded into a common latent space defined by the same set of network parameters, while still allowing view-specific normalization. 
The pre-training stage involves a contrastive loss on the audio-only and video-only paths, which pulls the audio and video representations from the same clip closer together in the joint space and pushes representations from different clips apart.
This architecture and training procedure jointly shape a unified and alignable audio-visual representation space, which serves as the basis for our subsequent contrastive correction and probabilistic modeling.

On top of this backbone, we focus on the TTA stage, where different modalities may undergo distribution shifts of different severity. 
To handle this, we adopt an adaptive contrastive asymmetry rectification mechanism that naturally aligns with the design of the backbone. 
During the forward pass, both modalities are processed by their private encoders and the shared joint encoder, producing global representations that lie in the same representation space. 
We then impose contrastive constraints to promote cross-modal alignment and intra-modal consistency. 

In our probabilistic formulation, we assume that the multi-modal feature, the audio feature, and the video feature, each obtained by mean-pooling the global representations from the joint encoder $\mathcal{F}$, are variables in the same latent feature space. It is therefore natural to impose the same form of distributional prior on all of them.

% \section*{C. More Experimental Results}

\section*{C. More Visualization Results}
\paragraph{Discussion of Covariance Matrices.} To further justify the use of category-specific covariance matrices rather than a single shared covariance matrix, we visualize in Fig.~\ref{fig:cov} the covariance structures estimated by our Gaussian model. For clarity, we compare the covariance matrix of each category with the average covariance matrix $\bar{\boldsymbol{\Sigma}}$ over all categories and examine their deviations $\boldsymbol{\Sigma}_c - \bar{\boldsymbol{\Sigma}}$. 
The resulting deviation maps exhibit highly structured patterns: certain rows, columns, and sub-blocks systematically deviate from the mean covariance, and these patterns vary markedly across categories. 
In other words, different categories are not only centered at different mean locations, but also differ in how variance and inter-dimensional correlations are distributed across the feature space. 
Such category-dependent correlation structures cannot be captured by a single shared covariance matrix. Therefore, introducing category-specific covariance matrices $\{\boldsymbol{\Sigma}_c\}_c$ is necessary to faithfully model the category-conditional densities.

\clearpage
